# Supplementary material for: HF-Fed: Hierarchical based customized Federated Learning Framework for X-Ray Imaging
Source: arXiv:2407.17780 source file (2024-07-25)
Supplement: Supplementary file 1 [file supplementary.tex]

\begin{center}
{\Large Supplementary material for Paper ID: 1343}
\end{center}

\begin{table}[H]
    \centering
    \caption{Below are the detailed hyper-parameters corresponding to each benchmark, with the source dataset as the In-house dataset}
    \label{tab:implementation_details}
    \begin{adjustbox}{width=\textwidth}
    \begin{tabular}{@{}clcc@{}}
        \toprule
        \textbf{Hyper-parameter} & \textbf{Description} & \textbf{INBreast} & \textbf{DDSM}  \\
        \midrule
       $N_c$ & Number of categories for classification head  & 2 & 2  \\
        $N_l^{\text{enc}}$& Number of encoder layers  & 8 & 6  \\
        $N_l^{\text{dec}}$ & Number of decoder layers   & 8 & 6   \\
        $N_l^{\text{aux}}$ &Number of MAE auxiliary decoder layers  & 2& 2  \\
        $N_q^{\text{dec}}$ & Number of queries for decoder   & 300 & 300 \\
        $N_q^{\text{aux}}$ &Number of queries for MAE auxiliary decoder & 882  & 882\\
        $H$& Number of hidden dimension for deformable attention& 256 &  256\\
        $F$ & Number of feedforward dimension for deformable attention   & 1024 &1024 \\
        $L$ & Number of feature levels for deformable attention   & 4& 4  \\
        $M$ & Number of heads for deformable attention & 8& 8\\
        $K$ & Number of reference points for each attention head& 4 & 4 \\
        % $dropout$& Ratio for dropout in Deformable DETR   & 0.0& 0.0 & 0.0\\
        $B$ & Batch Size during training   & 16 &16   \\
        $lr$ & Learning rate for modules except backbone and projection   & $2 \times 10^{-4}$&$ 2 \times 10^{-4}$\\
        $lr_{bac}$ & Learning rate for backbone and projection modules   & $2 \times 10^{-5}$ & $2 \times 10^{-5}$ \\
        $\beta_{bac}$ & Coefficient of discrimination loss after backbone $L_{\text{bac}}^{\text{dis}}$& 0.3 & 0.3 \\
        $\beta_{enc}$ & Coefficient of discrimination loss after encoder $L_{\text{enc}}^{\text{dis}}$
 & 1.0 &  1.0 \\
        $\beta_{dec}$ &Coefficient of discrimination loss after decoder $L_{\text{enc}}^{\text{dis}}$
 &  1.0 &  1.0 \\
        $\lambda_{unsup}$ & Coefficient of unsupervised loss $\mathcal{L}_{unsup}$ &  1.0 &  1.0 \\
        $\lambda_{mask}$ & Coefficient of supervised loss $\mathcal{L}_{sup}$ &  1.0 &  1.0\\
        $\gamma$ & EMA update ratio & 0.9996 & 0.9996 \\
        $\mu_{t}$ & Initial Mask ratio in MAE branch & 0.2 & 0.3 \\
        $\eta$ & Initial step for annealing & 0.2 & 0.3 \\

        $\eta^i_{min}$ & Minimum jump in mask annealing step $\eta$ & 0.05 & 0.05 \\
        $\eta^i_{max}$ & Maximum jump in mask annealing step $\eta$ & 0.15 & 0.15 \\
        $C_s$&Soft Confidence Metric&0.15&0.20\\
        $C_h$&Hard Confidence Metric&0.80&0.90\\\
        $E_{pre}$ & MAE branch with source data training epoch number & 88 & 87  \\
        $E_{teach}$ & Teacher-student training epoch number & 84 & 76 \\
        $E_{decay}$ & After Edecay epochs in teaching stage, we drop the MAE branch & 30 & 10\\
        $E_{reinit}$ & Re-initialization epoch for selective retraining & 40 & 20 \\
        
        \bottomrule
    \end{tabular}
    \end{adjustbox}
\end{table}
 %hyperparameters
\begin{table*}[hbtp]
\centering
  \resizebox{\linewidth}{!}{
    \begin{tabular}{@{}c|l|l|cccccc|cc@{}}
    \toprule
    \textbf{Datasets}& \makecell[c]{\textbf{Model Name}} & \makecell[c]{\textbf{Venue}} & \textbf{R@0.05} & \textbf{R@0.1} & \textbf{R@0.3} &\textbf{R@0.5}& \textbf{R@1.0} & \textbf{R@2.0} & \textbf{Accuracy} & \textbf{F1-score} \\ \midrule
    & SFA\cite{wang2021exploring} & MM'21&0.01 & 0.01& 0.05& 0.07& 0.11&0.313 & 0.216&0.329\cr
    & UMT\cite{deng2021unbiased} & CVPR'21 &0.0 & 0.01&0.04 & 0.07& 0.09&0.13 & 0.261&0.362\cr
    & D-Adapt\cite{jiang2021decoupled} & ICLR'22 &0.0 & 0.02& 0.06&0.09 &0.10 &0.13 &0.382 &0.215\cr
    & AT\cite{li2022cross} & CVPR'22 & 0.01& 0.03&0.08 &0.10 &0.15 & 0.21&0.216 & 0.311\cr
    \textbf{\texttt{In-house} to} & H2FA\cite{xu2022h2fa} & CVPR'22 &0.02 & 0.03&0.06 &0.10 & 0.12&0.17 &0.371&0.315 \cr
    \textbf{\ddsm~\cite{lee2017curated}} & AQT\cite{huang2022aqt} & IJCAI'22 &0.01 &0.03 & 0.07& 0.13& 0.15&0.18 &0.412&0.398\cr
    & HT\cite{deng2023harmonious}  & CVPR'23 & 0.03&0.05&0.08 &0.10 &0.13 & 0.15&0.362&0.362 \cr
    & ConfMIX\cite{mattolin2023confmix} & WACV'23& 0.02&0.04 &0.09 &0.12 &0.16 &0.19 &0.336 &0.412\cr
    & CLIPGAP\cite{vidit2023clip} & CVPR'23 &0.01& 0.03& 0.07& 0.11& 0.15& 0.16& 0.336& 0.458\cr
    & MRT\cite{zhao2023masked} & ICCV'23 &0.03& 0.04& 0.09&0.12 & 0.17& 0.21&0.421 &0.587 \cr
    & \textbf{Ours} &- & \textbf{0.02}& \textbf{0.05} & \textbf{0.12} & \textbf{0.17} & \textbf{0.29} & \textbf{0.49}&\textbf{0.561}&\textbf{0.613} \cr \midrule
    & SFA\cite{wang2021exploring} & MM'21& 0.03& 0.07&0.13 &0.18 & 0.27&0.31& 0.629&0.210\cr
    & UMT\cite{deng2021unbiased} & CVPR'21  & 0.01&0.04& 0.09&0.15 &0.19 &0.23 &0.568&0.193\cr
    & D-Adapt\cite{jiang2021decoupled} & ICLR'22&0.03 &0.06 & 0.11& 0.18&0.25 &0.31 &0.668&0.241 \cr
    & AT\cite{li2022cross} & CVPR'22  & 0.10&0.28& 0.37& 0.45& 0.51& 0.66&0.725&\textbf{0.319}\cr
    \textbf{\rsna to} & H2FA\cite{xu2022h2fa} &CVPR'22& 0.03& 0.06& 0.14& 0.17&0.21 & 0.24& 0.591&0.274 \cr
    \textbf{\texttt{In-house}} & AQT\cite{huang2022aqt} &IJCAI'22&0.01 &0.05 &0.08 & 0.11& 0.17& 0.20& 0.527&0.230 \cr
    & HT\cite{deng2023harmonious}  & CVPR'23 &0.02& 0.10& 0.17&0.24 &0.33 & 0.41& 0.710&0.291\cr
    & ConfMIX\cite{mattolin2023confmix} & WACV'23 &0.03& 0.09&.0.16 &0.28 & 0.35& 0.39& 0.622&0.263 \cr
    & CLIPGAP\cite{vidit2023clip} & CVPR'23 &0.04& 0.08&0.23 & 0.36&0.64 &0.72 & 0.797&0.231\cr
    & MRT\cite{zhao2023masked} & ICCV'23 &0.06 & 0.11&0.29 &0.44 & 0.65&0.76 & 0.825& 0.304\cr
    & \textbf{Ours} & &  \textbf{0.14} & \textbf{0.20} & \textbf{0.37} & \textbf{0.54} & \textbf{0.72} & \textbf{0.83} & \textbf{0.825}&0.312 \cr \bottomrule
    \end{tabular}
  }
  \vspace{0.2em}
  \caption{\cref{tab:sota_uda_comparison} in the main paper showed similar comparison with \sota \uda methods on few dataset pairs. Here we show results for few more pairs.}
  \label{tab:sota_uda_comparison_suppl}

\end{table*} %comparison with uda

\begin{figure}[htbp]
\centering
\begin{subfigure}[b]{0.15\textwidth}
  {\centering\caption{\texttt{In-house}}}
  \vspace{0.95cm}
\end{subfigure}
\hfill
\begin{subfigure}[b]{0.16\textwidth}
    \includegraphics[height=2.1cm, width= 2 cm]{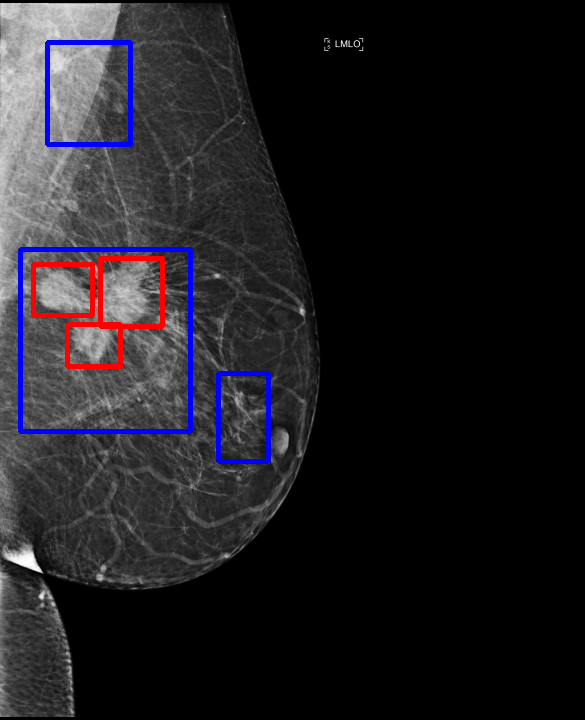}
\end{subfigure}
\hfill
\begin{subfigure}[b]{0.16\textwidth}
    \includegraphics[height=2.1cm, width= 2 cm]{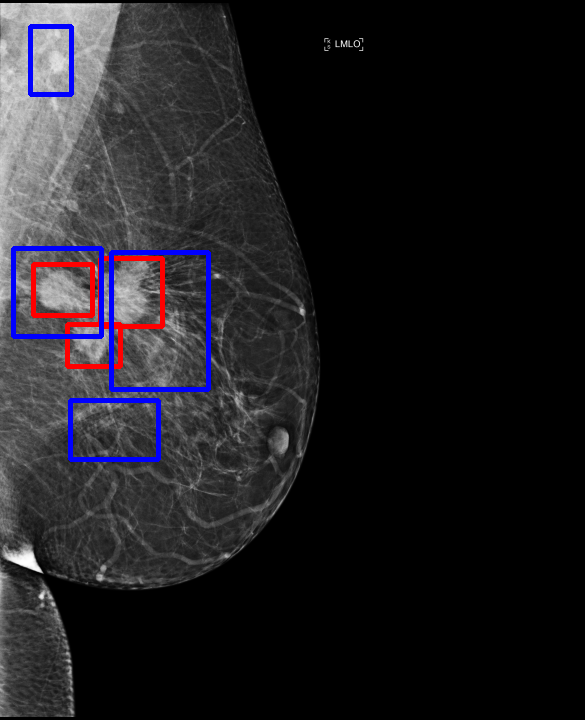}
\end{subfigure}
\hfill
\begin{subfigure}[b]{0.16\textwidth}
    \includegraphics[height=2.1cm, width= 2 cm]{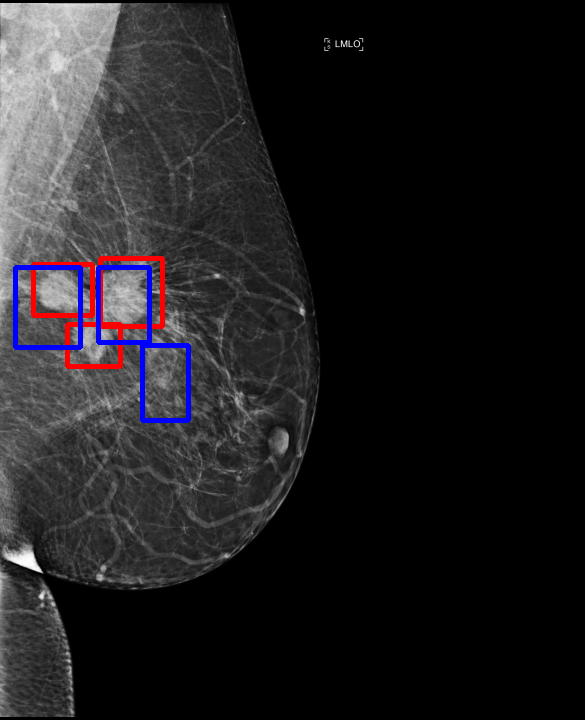}
\end{subfigure}
\hfill
\begin{subfigure}[b]{0.16\textwidth}
    \includegraphics[height=2.1cm, width= 2 cm]{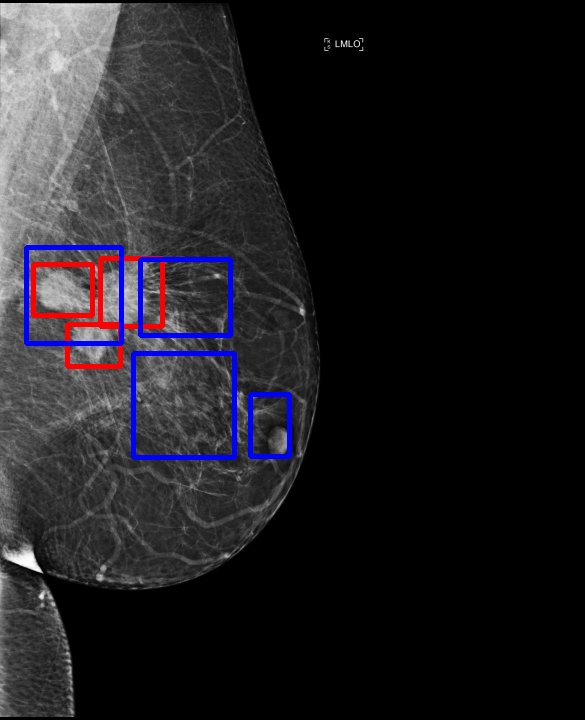}
\end{subfigure}
\hfill
\begin{subfigure}[b]{0.16\textwidth}
    \includegraphics[height=2.1cm, width= 2 cm]{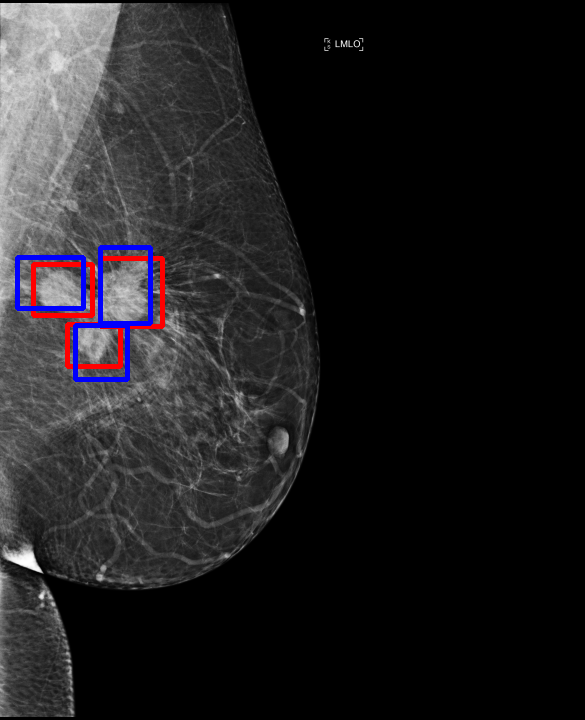}
\end{subfigure}
\vspace{-0.02em}
\begin{subfigure}[b]{0.15\textwidth}
  {\centering\caption{\ddsm~\cite{lee2017curated}}}
  \vspace{0.95cm}
\end{subfigure}
\hfill
\begin{subfigure}[b]{0.16\textwidth}
    \includegraphics[height=2.1cm, width= 2 cm]{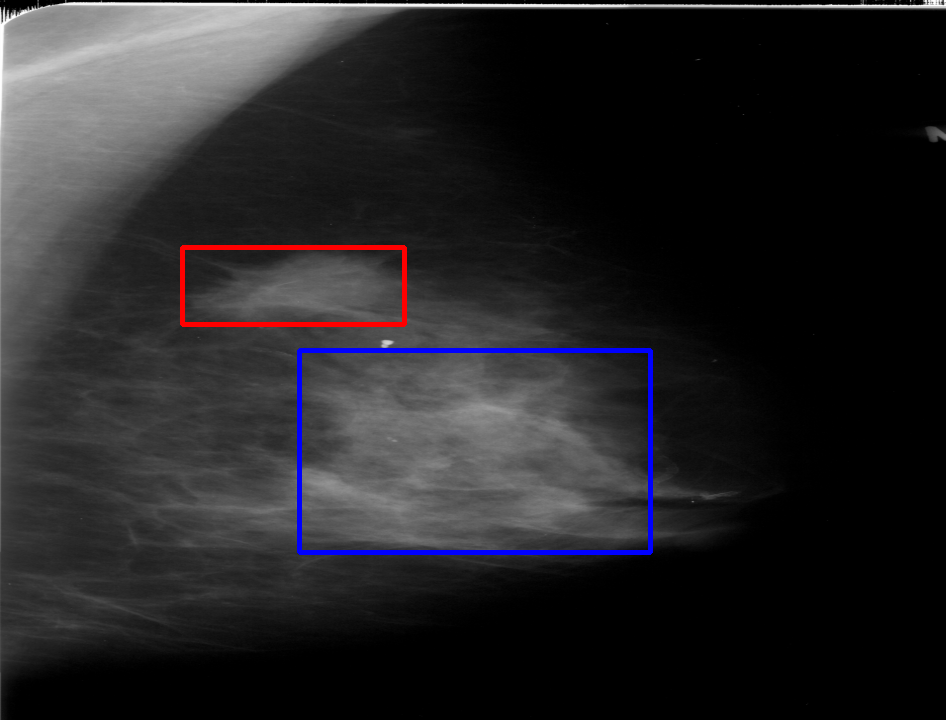}
\end{subfigure}
\hfill
\begin{subfigure}[b]{0.16\textwidth}
    \includegraphics[height=2.1cm, width= 2 cm]{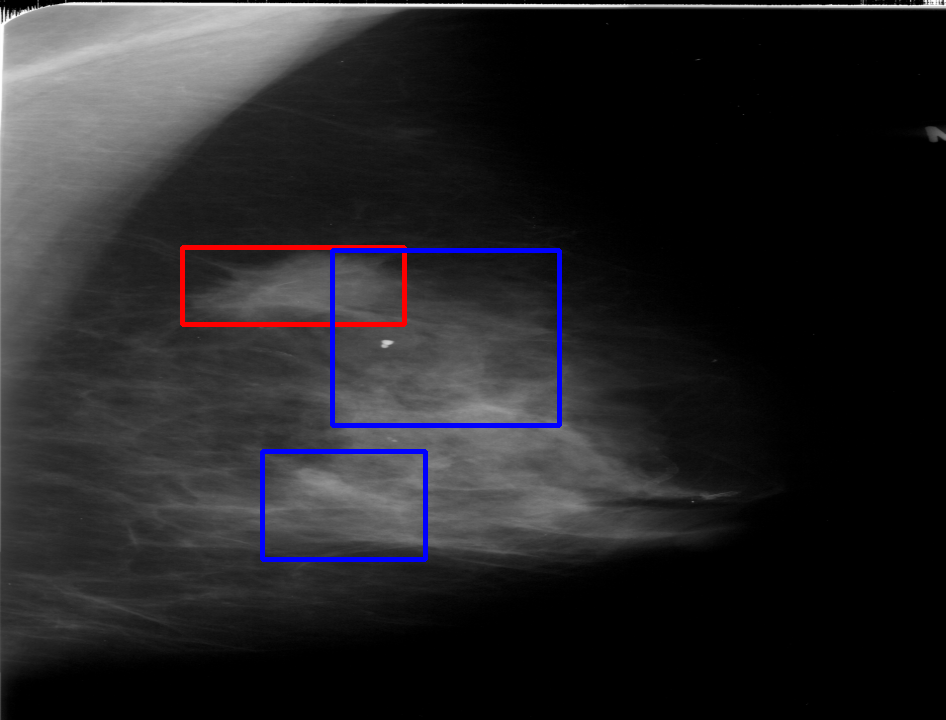}
\end{subfigure}
\hfill
\begin{subfigure}[b]{0.16\textwidth}
    \includegraphics[height=2.1cm, width= 2 cm]{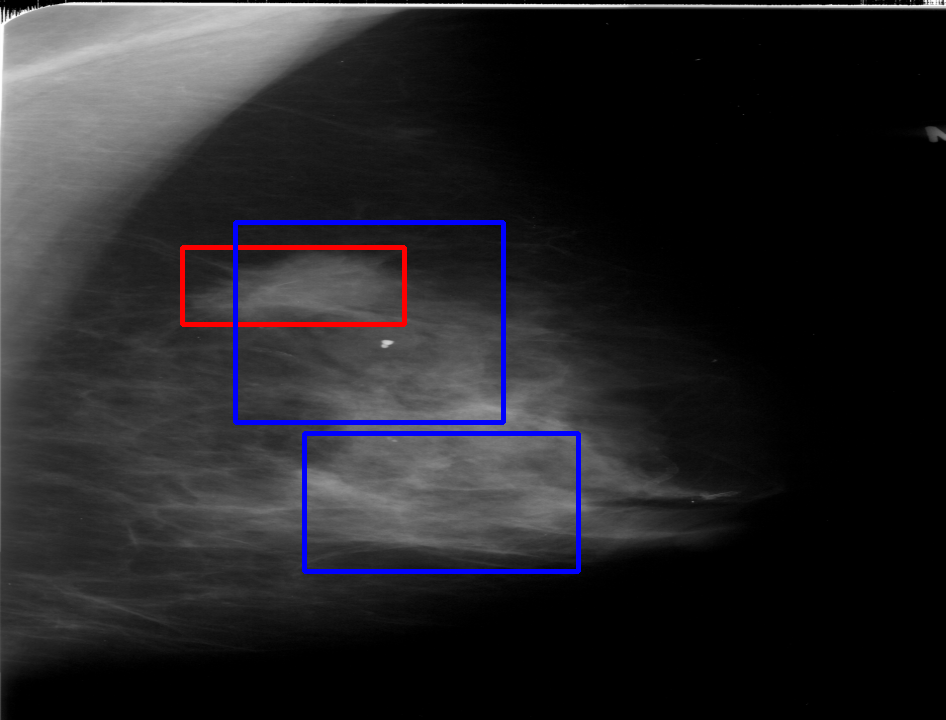}
\end{subfigure}
\hfill
\begin{subfigure}[b]{0.16\textwidth}
    \includegraphics[height=2.1cm, width= 2 cm]{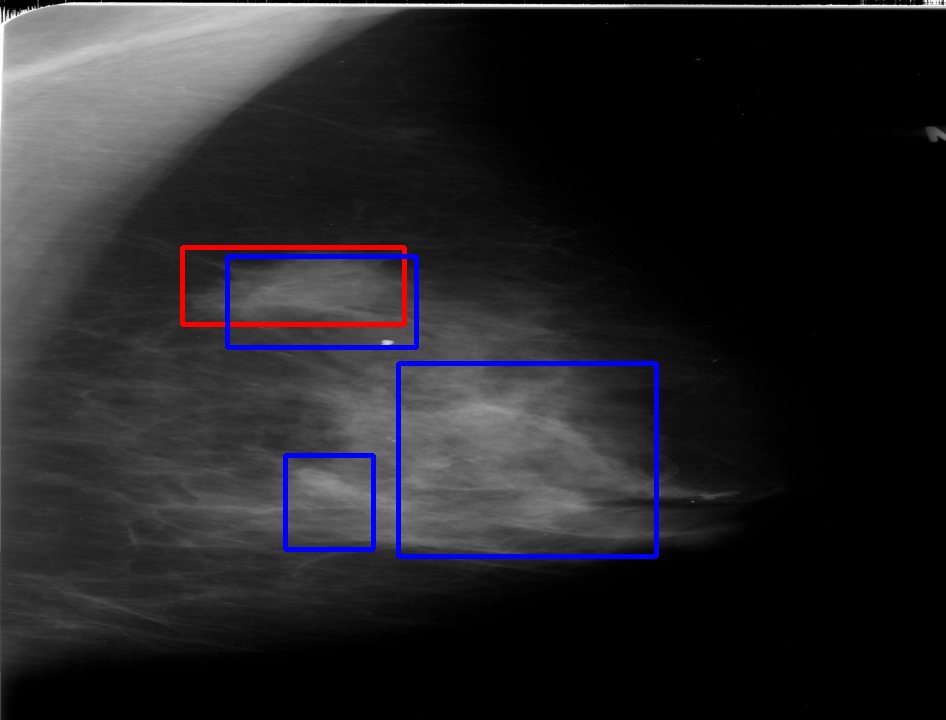}
\end{subfigure}
\hfill
\begin{subfigure}[b]{0.16\textwidth}
    \includegraphics[height=2.1cm, width= 2 cm]{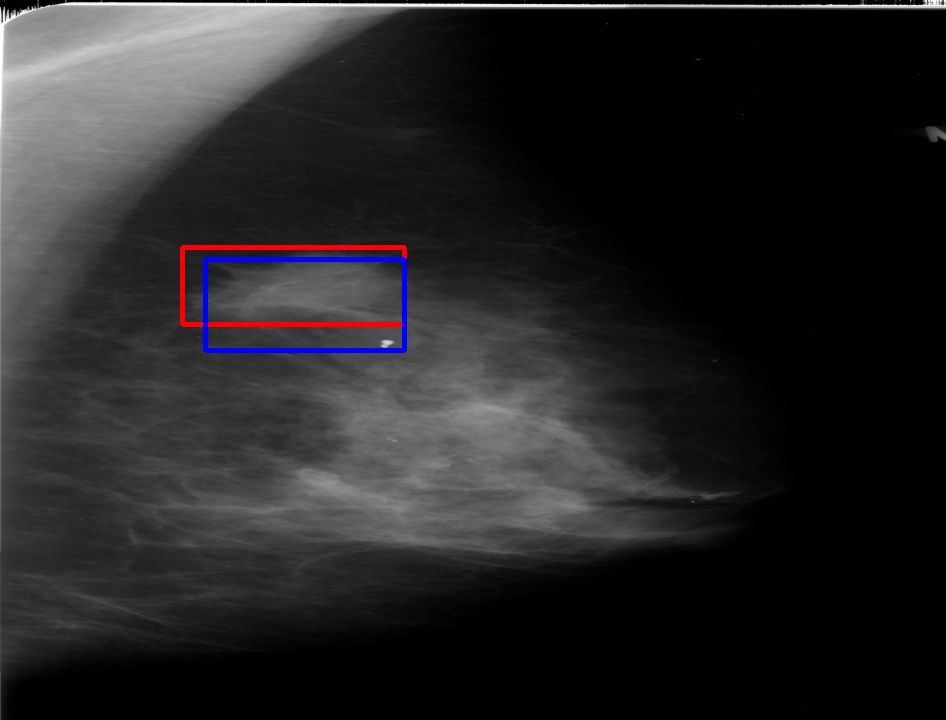}
\end{subfigure}
\vspace{-0.01em}
\begin{subfigure}[b]{0.15\textwidth}
  {\centering\caption{\rsna}}
  \vspace{1.55cm}
\end{subfigure}
\hfill
\begin{subfigure}[b]{0.16\textwidth}
    \includegraphics[height=2.1cm, width=2cm]{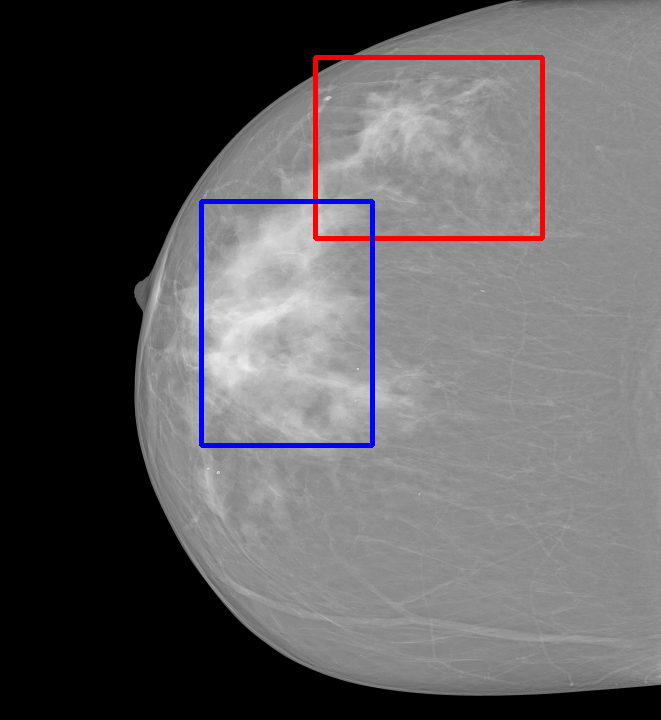}
    \caption{Source}
\end{subfigure}
\hfill
\begin{subfigure}[b]{0.16\textwidth}
    \includegraphics[height=2.1cm, width=2cm]{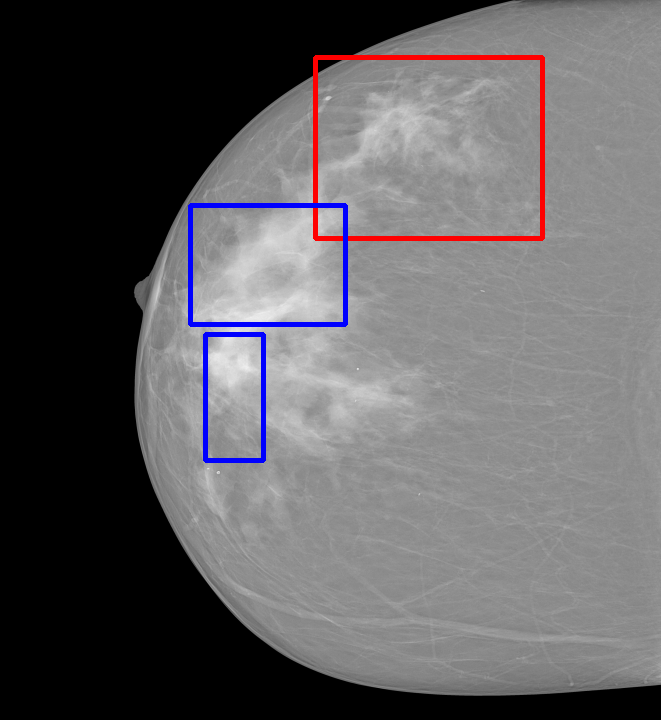}
    \caption{AT~\cite{li2022cross}}
\end{subfigure}
\hfill
\begin{subfigure}[b]{0.16\textwidth}
    \includegraphics[height=2.1cm, width=2cm]{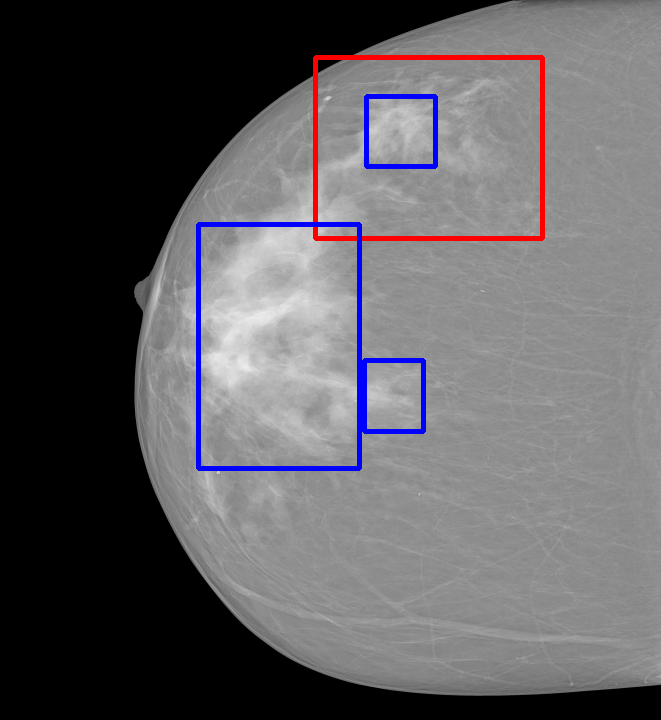}
    \caption{MRT~\cite{zhao2023masked}}
\end{subfigure}
\hfill
\begin{subfigure}[b]{0.16\textwidth}
    \includegraphics[height=2.1cm, width=2cm]{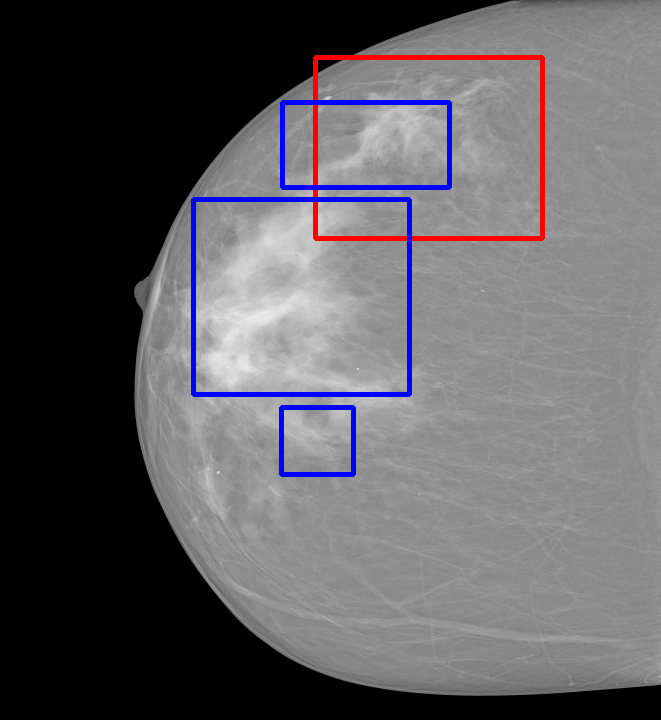}
    \caption{HT~\cite{deng2023harmonious}}
\end{subfigure}
\hfill
\begin{subfigure}[b]{0.16\textwidth}
    \includegraphics[height=2.1cm, width=2cm]{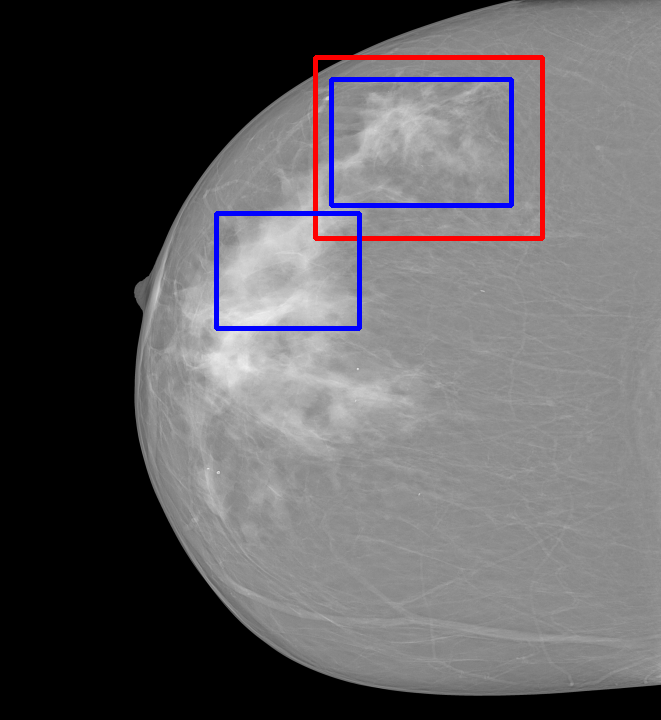}
    \caption{Ours}
\end{subfigure}
\caption{Qualitative result comparison on in-house, \ddsm, and \rsna datasets. Red boxes show the ground truth, and blue boxes show the predictions.}
\label{fig:qualitative_results}
\end{figure}
 %qualitative results
%\input{tables/table3}
